# Supplementary material for: QuantumFed: A Federated Learning Framework for Collaborative Quantum Training
Source: arXiv:2106.09109 source file (2022-06-29)
Supplement: Supplementary file 1 [file appendix.tex]

\appendix

\section{Proof of Proposition~\ref{computeK}}

\begin{proof}
    Assume $\mathcal{C}(s)=\mathcal{C}(U,(\phi_{n,x}^{in},\phi_{n,x}^{out}))$, $\mathcal{C}(s+\epsilon)=\mathcal{C}(e^{i\epsilon K}U, (\phi_{n,x}^{in},\phi_{n,x}^{out}))$ to represent the cost function before and after the local update respectively, and $\rho_x^{out}(s), \rho_x^{out}(s+\epsilon)$ are defined likewise, by Taylor's expansion, we have:
    \begin{align*}
        &\rho_x^{out}(s+\epsilon)\\
        =&\text{tr}_{in,hidden}(e^{i\epsilon K_{m_{out}}^{out}}U_n^{out,m_{out}}(s)e^{i\epsilon K_{m_{out}-1}^{out}}U_n^{out,m_{out}-1}(s)\cdots e^{i\epsilon K_{1}^{1}}U_n^{1,1}(s)(\rho_x^{in}\otimes|0\cdots0\rangle_{hidden,out}\langle0\cdots0|){U_n^{1,1}}^{\dagger}\\
        &e^{-i\epsilon K_1^1}\cdots{U_n^{out,m_{out}}}^{\dagger}e^{-i\epsilon K_{m_{out}}^{out}})\\
        =&\rho_x^{out}(s)+i\epsilon\text{tr}_{in,hidden}(K_{m_{out}}^{out}U_n^{out,m_{out}}(s)\cdots U_n^{1,1}(s)(\rho_x^{in}\otimes|0\cdots0\rangle_{hidden,out}\langle0\cdots0|){U_n^{1,1}}^{\dagger}(s)\cdots{U_n^{out,m_{out}}}^{\dagger}(s))\\
        &-U_n^{out,m_{out}}(s)\cdots U_n^{1,1}(s)(\rho_x^{in}\otimes|0\cdots0\rangle_{hidden,out}\langle0\cdots0|){U_n^{1,1}}^{\dagger}(s)\cdots{U_n^{out,m_{out}}}^{\dagger}(s){K_{m_{out}}^{out}}+\cdots\\
        &+U_n^{out,m_{out}}(s)\cdots K_1^1U_n^{1,1}(s)(\rho_x^{in}\otimes|0\cdots0\rangle_{hidden,out}\langle0\cdots0|){U_n^{1,1}}^{\dagger}(s)\cdots{U_n^{out,m_{out}}}^{\dagger}(s)\\
        &-U_n^{out,m_{out}}(s)\cdots U_n^{1,1}(s)(\rho_x^{in}\otimes|0\cdots0\rangle_{hidden,out}\langle0\cdots0|){U_n^{1,1}}^{\dagger}(s)K_1^1\cdots{U_n^{out,m_{out}}}^{\dagger}(s))+O(\epsilon^2)\\
        =&\rho_x^{out}(s)+i\epsilon\text{tr}_{in,hidden}([K_{m_{out}}^{out}, U_n^{out,m_{out}}(s)\cdots U_n^{1,1}(s)(\rho_x^{in}\otimes|0\cdots0\rangle_{hidden,out}\langle0\cdots0|){U_n^{1,1}}^{\dagger}(s)\cdots{U_n^{out,m_{out}}}^{\dagger}(s)]\\
        &+\cdots+U_n^{out,m_{out}}(s)\cdots U_n^{1,2}(s)[K_1^1,U_n^{1,1}(s)(\rho_x^{in}\otimes|0\cdots0\rangle_{hidden,out}\langle0\cdots0|){U_n^{1,1}}^{\dagger}(s)]{U_n^{1,2}}^{\dagger}(s)\cdots{U_n^{out,m_{out}}}^{\dagger}(s))+O(\epsilon^2)
    \end{align*}
    Here $\rho_{x}^{in}=|\phi_{n,x}^{in}\rangle\langle\phi_{n,x}^{in}|$.
    Then we can compute the derivative of cost function as:
    \begin{align*}
        &\frac{d\mathcal{C}(s)}{ds}=\lim_{\epsilon\rightarrow0}\frac{\mathcal{C}(s+\epsilon)-\mathcal{C}}{\epsilon}\\
        =&\lim_{\epsilon\rightarrow0}\frac{\mathcal{C}(s)\frac{i\epsilon}{N_n}\sum_{x=1}^{N_n}\langle\phi_{n,x}^{out}|\text{tr}_{in,hidden}(\rho_x^{out}(s+\epsilon))|\phi_{n,x}^{out}\rangle-\mathcal{C}(s)}{\epsilon}\\
        =&\frac{1}{N_n}\sum_{x=1}^{N_n}(\mathbb{I}_{in,hidden}\otimes|\phi_{n,x}^{out}\rangle\langle\phi_{n,x}^{out}|([iK_{m_{out}}^{out},U_n^{out,m_{out}}(s)\cdots U_n^{1,1}(s)(\rho_x^{in}\otimes|0\cdots0\rangle_{hidden,out}\langle0\cdots0|){U_n^{1,1}}^{\dagger}(s)\cdots{U_n^{out,m_{out}}}^{\dagger}(s)]\\
        &+\cdots+U_n^{out,m_{out}}(s)\cdots U_n^{1,2}(s)[iK_1^1,U_n^{1,1}(s)(\rho_x^{in}\otimes|0\cdots0\rangle_{hidden,out}\langle0\cdots0|){U_n^{1,1}}^{\dagger}(s)]{U_n^{1,2}}^{\dagger}(s)\cdots{U_n^{out,m_{out}}}^{\dagger}(s)))\\
        =&\frac{1}{N_n}\sum_{x=1}^{N_n}\text{tr}([U_n^{out,m_{out}}(s)\cdots U_n^{1,1}(s)(\rho_{n,x}^{in}\otimes|0\cdots0\rangle_{hidden,out}\langle0\cdots0|){U_n^{1,1}}^{\dagger}(s)\cdots{U_n^{out,m_{out}}}^{\dagger}(s),\mathbb{I}_{in,hidden}\otimes|\phi_{n,x}^{out}\rangle\langle\phi_{n,x}^{out}|]\\
        &iK_{m_{out}}^{out}+\cdots+[U_n^{1,1}(s)(\rho_{n,x}^{in}\otimes|0\cdots0\rangle_{hidden,out}\langle0\cdots0|){U_n^{1,1}}^{\dagger}(s),{U_n^{1,2}}^{\dagger}(s)\cdots{U_n^{out,m_{out}}}^{\dagger}(s)(\mathbb{I}_{in,hidden}\otimes|\phi_{n,x}^{out}\rangle\langle\phi_{n,x}^{out}|)\\
        &U_n^{out,m_{out}}(s)\cdots U_n^{1,2}(s)]iK_1^1)\\
        =&\frac{i}{N_n}\sum_{x=1}^{N_n}\text{tr}(M_x^{out,m_{out}}K_{m_{out}}^{out}+\cdots+M_x^{1,1}K_1^1)
    \end{align*}
    This is given by the property that the trace of a product can be switched without changing the result. Here we let $M_x^{l,j}=[\prod_{\alpha=j}^1U_{n}^{l,\alpha}(\rho_{x}^{l-1}\otimes|0\cdots0\rangle_l\langle 0\cdots0|)\prod_{\alpha=1}^j{U_{n}^{l,\alpha}}^{\dagger},\prod_{\alpha=j+1}^{m_l}{U_{n}^{l,\alpha}}^{\dagger}(\mathbb{I}_{l-1}\otimes\sigma_{x}^l)\prod_{\alpha=m_l}^{j+1}U_{n}^{l,\alpha}]$ and $\mathcal{F}^l$ is the adjoint channel to $\mathcal{E}^l$ and $\sigma_x^l=\mathcal{F}^{l+1}(\cdots\mathcal{F}^{out}(|\phi_{n,x}^{out}\rangle\langle\phi_{n,x}^{out}|))$.
    
    Let $\alpha_i$ denote each qubit in the previous layer and $\beta$ denote the current qubit in the current layer. We also denote $\sigma$ as the Pauli matrices. Then we can assume:
    \begin{equation*}
        K_j^l=\sum_{\alpha_1,\cdots,\alpha_{m_{l-1}},\beta}k_{j,\alpha_1,\cdots,\alpha_{m_{l-1}}}^l(\sigma^{\alpha_1}\otimes\cdots\otimes\sigma^{\alpha_{m_{l-1}}}\otimes\sigma^{\beta})
    \end{equation*}
    Because we would like to maximize (\ref{defineK}), using gradient ascent, we would like to maximize the gradient to get the fastest growth direction with the condition of bounded $K$. Therefore, we would like to optimize $K$ for:
    \begin{align*}
        K=&\arg\max_{K}(\frac{d\mathcal{C}(s)}{ds}-\lambda'\sum_{\alpha_i,beta}{k_{j,\alpha_1,\cdots,\alpha_{m_{l-1}}}^l}^2)\\
        =&\arg\max_{K}(\frac{i}{N_n}\sum_{x=1}^{N_n}\text{tr}(M_x^{out,m_{out}}K_{m_{out}}^{out}+\cdots+M_x^{1,1}K_1^1)-\lambda'\sum_{\alpha_i,beta}{k_{j,\alpha_1,\cdots,\alpha_{m_{l-1}}}^l}^2)\\
        =&\arg\max_{K}(\frac{i}{N_n}\sum_{x=1}^{N_n}\text{tr}_{\alpha_i,\beta}(\text{tr}_{rest}(M_x^{out,m_{out}}K_{m_{out}}^{out}+\cdots+M_x^{1,1}K_1^1))-\lambda'\sum_{\alpha_i,beta}{k_{j,\alpha_1,\cdots,\alpha_{m_{l-1}}}^l}^2)\\
    \end{align*}
    Let the derivative of $k_{j,\alpha_1,\cdots,\alpha_{m_{l-1}}}^l$ equals to $0$, we have:
    \begin{equation*}
        \frac{i}{N_n}\sum_{x=1}^{N_n}\text{tr}_{\alpha_i,\beta}(\text{tr}_{rest}(M_x^{l,j})(\sigma^{\alpha_1}\otimes\cdots\otimes\sigma^{\alpha_{m_{l-1}}}\otimes\sigma^{\beta}))-2\lambda'k_{j,\alpha_1,\cdots,\alpha_{m_{l-1}}}^l=0
    \end{equation*}
    This is equivalent to:
    \begin{equation*}
        k_{j,\alpha_1,\cdots,\alpha_{m_{l-1}}}^l=\frac{i}{2N_n\lambda'}\sum_{x=1}^{N_n}\text{tr}_{\alpha_i,\beta}(\text{tr}_{rest}(M_x^{l,j})(\sigma^{\alpha_1}\otimes\cdots\otimes\sigma^{\alpha_{m_{l-1}}}\otimes\sigma^{\beta}))
    \end{equation*}
    Then we can derive $K_j^l$:
    \begin{align*}
        K_j^l=&\sum_{\alpha_i,\beta}k_{j,\alpha_1,\cdots,\alpha_{m_{l-1}}}^l(\sigma^{\alpha_1}\otimes\cdots\otimes\sigma^{\alpha_{m_{l-1}}}\otimes\sigma^{\beta})\\
        =&\frac{i}{2N_n\lambda'}\sum_{\alpha_i,\beta}\sum_{x=1}^{N_n}\text{tr}_{\alpha_i,\beta}(\text{tr}_{rest}(M_x^{l,j})(\sigma^{\alpha_1}\otimes\cdots\otimes\sigma^{\alpha_{m_{l-1}}}\otimes\sigma^{\beta}))(\sigma^{\alpha_1}\otimes\cdots\otimes\sigma^{\alpha_{m_{l-1}}}\otimes\sigma^{\beta})\\
        =&\eta\frac{2^{m_{l-1}}i}{N_n}\sum_{x=1}^{N_n}\text{tr}_{rest}(M_j^l)
    \end{align*}
    Here $\eta=\frac{1}{\lambda'}$ as the learning rate.
\end{proof}

\section{More Experiments}

\subsection{Comparison of Different Network Architectures}

In this section, we first compare the performance of different quantum network architectures. Because of the simulation limit of the computational resources, we only compare four architectures: [2, 2], [2, 3, 2], [1, 2, 1], [2, 3, 3, 2]. The results are shown in Figure~\ref{arch_comparison}.
\begin{figure}[htb]
    \centering
    \includegraphics[width=\columnwidth]{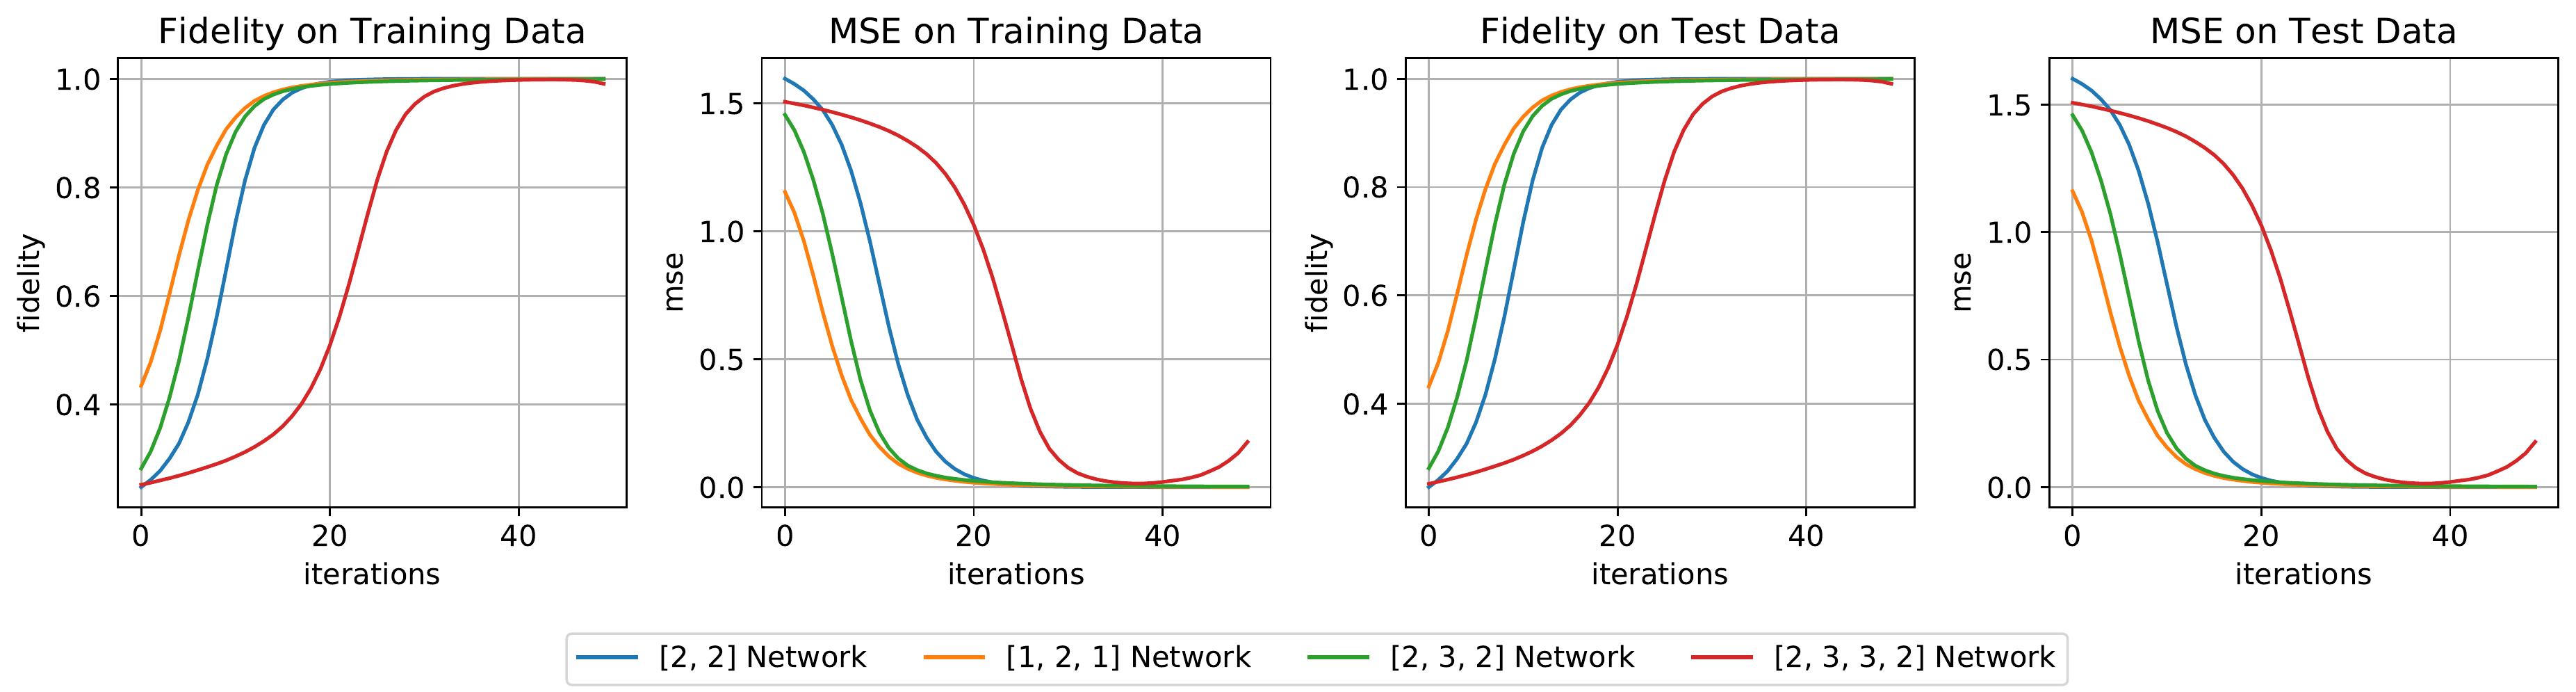}
    \caption{Experiment results of four different quantum networks.}
    \label{arch_comparison}
\end{figure}
It is easy to find that all four quantum networks are capable of having an acceptable performance in federated setting, while [2, 2], [2, 3, 2], [1, 2, 1] networks perform better than the [2, 3, 3, 2] network. This actually shows that in quantum neural networks, a larger sized network may not outperform a shallow network. Therefore, it is important to choose an appropriate network architecture to perform specific training tasks.

\subsection{Comparison of Different $\epsilon$ Choices}

In order to show the performance difference of different $\epsilon$ choices, we conduct experiences on a [2, 3, 2] network with $N=100$, $N_p=10$, $\eta=1.0$ and different $\epsilon$. The experiment results are in Figure~\ref{epsilon_comparison}.
\begin{figure}[htb]
    \centering
    \includegraphics[width=\columnwidth]{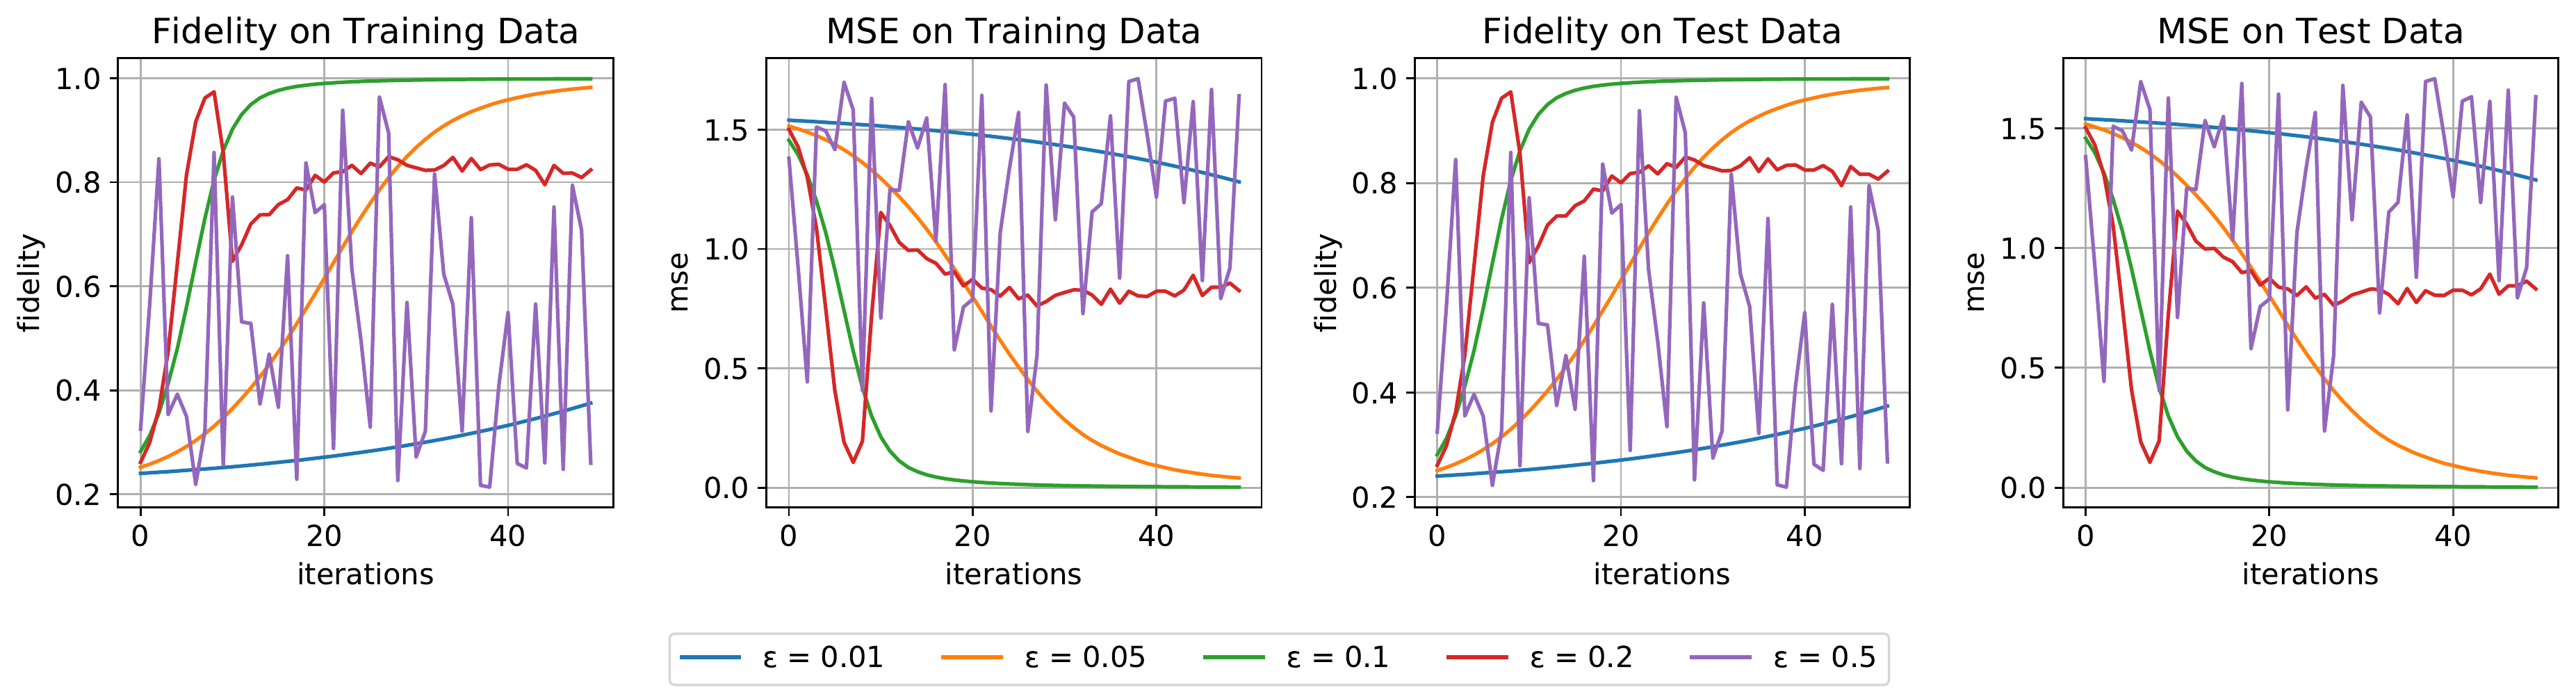}
    \caption{Experiment results of a [2, 3, 2] quantum networks with different $\epsilon$.}
    \label{epsilon_comparison}
\end{figure}
From this figure, we can find that when $\epsilon=0.1$ or $0.05$, the training approximates to the phase with fidelity of $1$ and MSE of $0$. When $\epsilon=0.01$, the training speed is really slow and the training does not converge after $50$ synchronization iterations. When $\epsilon=0.2$, the training speed outperforms training with smaller $\epsilon$ for first several iterations, but the performance downgrades a little bit in the following iterations and then keeps in a lower level. This may be caused by converging to other points. When $\epsilon=0.5$, it is obvious that the training does not converge. The performance changes back and forth in each iteration. This can be explained similar to the case in gradient descent. A larger step size will disturb the training and make each iteration go across the best point and not converge.

\subsection{Comparison of Different $\eta$ Choices}

We conduct similar experiments to compare how the choice of $\eta$ affects the performance of the training. We go through the experiments with the same parameter, same settings and different $\eta$ choices. The results are in Figure~\ref{lambda_comparison}.
\begin{figure}[htb]
    \centering
    \includegraphics[width=\columnwidth]{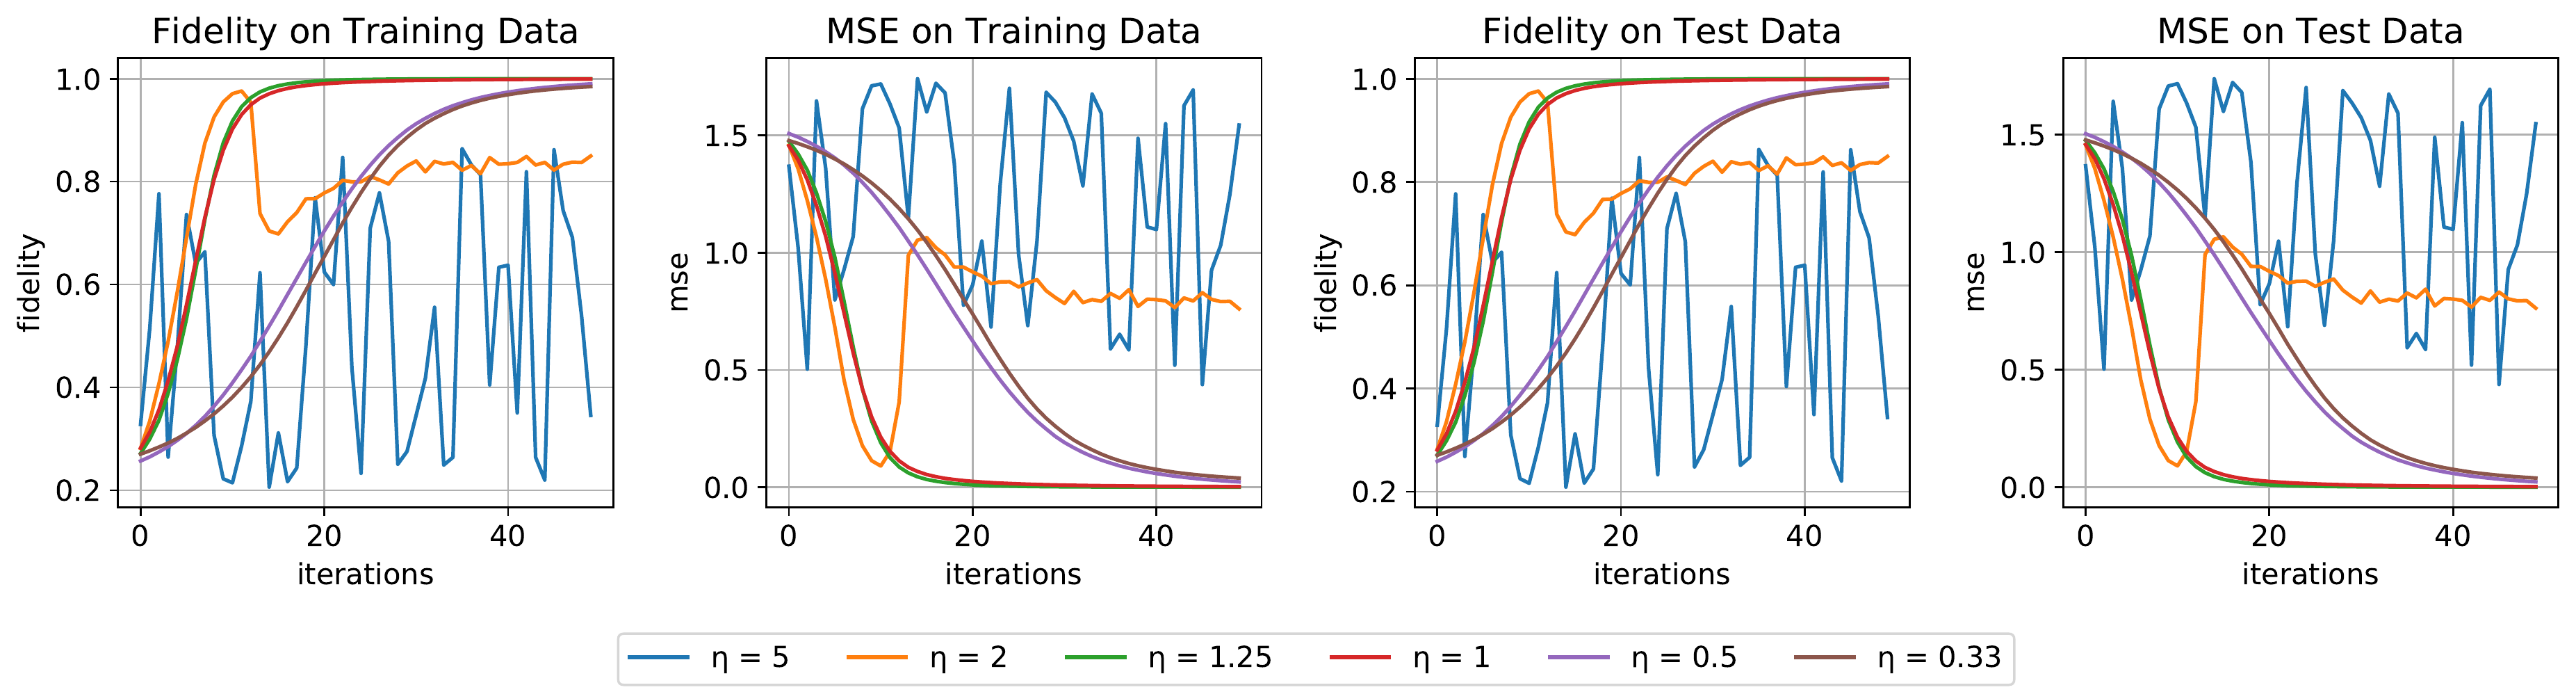}
    \caption{Experiment results of a [2, 3, 2] quantum network with different $\eta$.}
    \label{lambda_comparison}
\end{figure}
From this figure, we can find that when $\eta=1.0$ or $1.25$, the training has the fast convergence speed and best performance, while if we choose $\eta=0.5$ or $0.33$, the convergence speed declines a lot but still is acceptable. When $\eta$ chooses a relatively larger value, such as $2$ and $5$. The convergence will be misled to a wrong point. Here we can see that the choices of $\eta$ and $\epsilon$ have similar performance. In practice, we can fix the choice of $\eta$ and only adjust $\epsilon$ to get the best performance.

\subsection{Comparison of Different Proportions of Participants}

Here we choose different numbers of participants and different numbers of total nodes to figure out the influence of different proportions of participants. In order to show the difference, we conduct two experiments. First we set the total number of nodes to $10$ and change the number of participants. Then we fix the number of participants to $10$ and change the number of total nodes. The results are respectively in Figure~\ref{participants_comparison} and Figure~\ref{totalnodes_comparison}.
\begin{figure}[htb]
    \centering
    \includegraphics[width=\columnwidth]{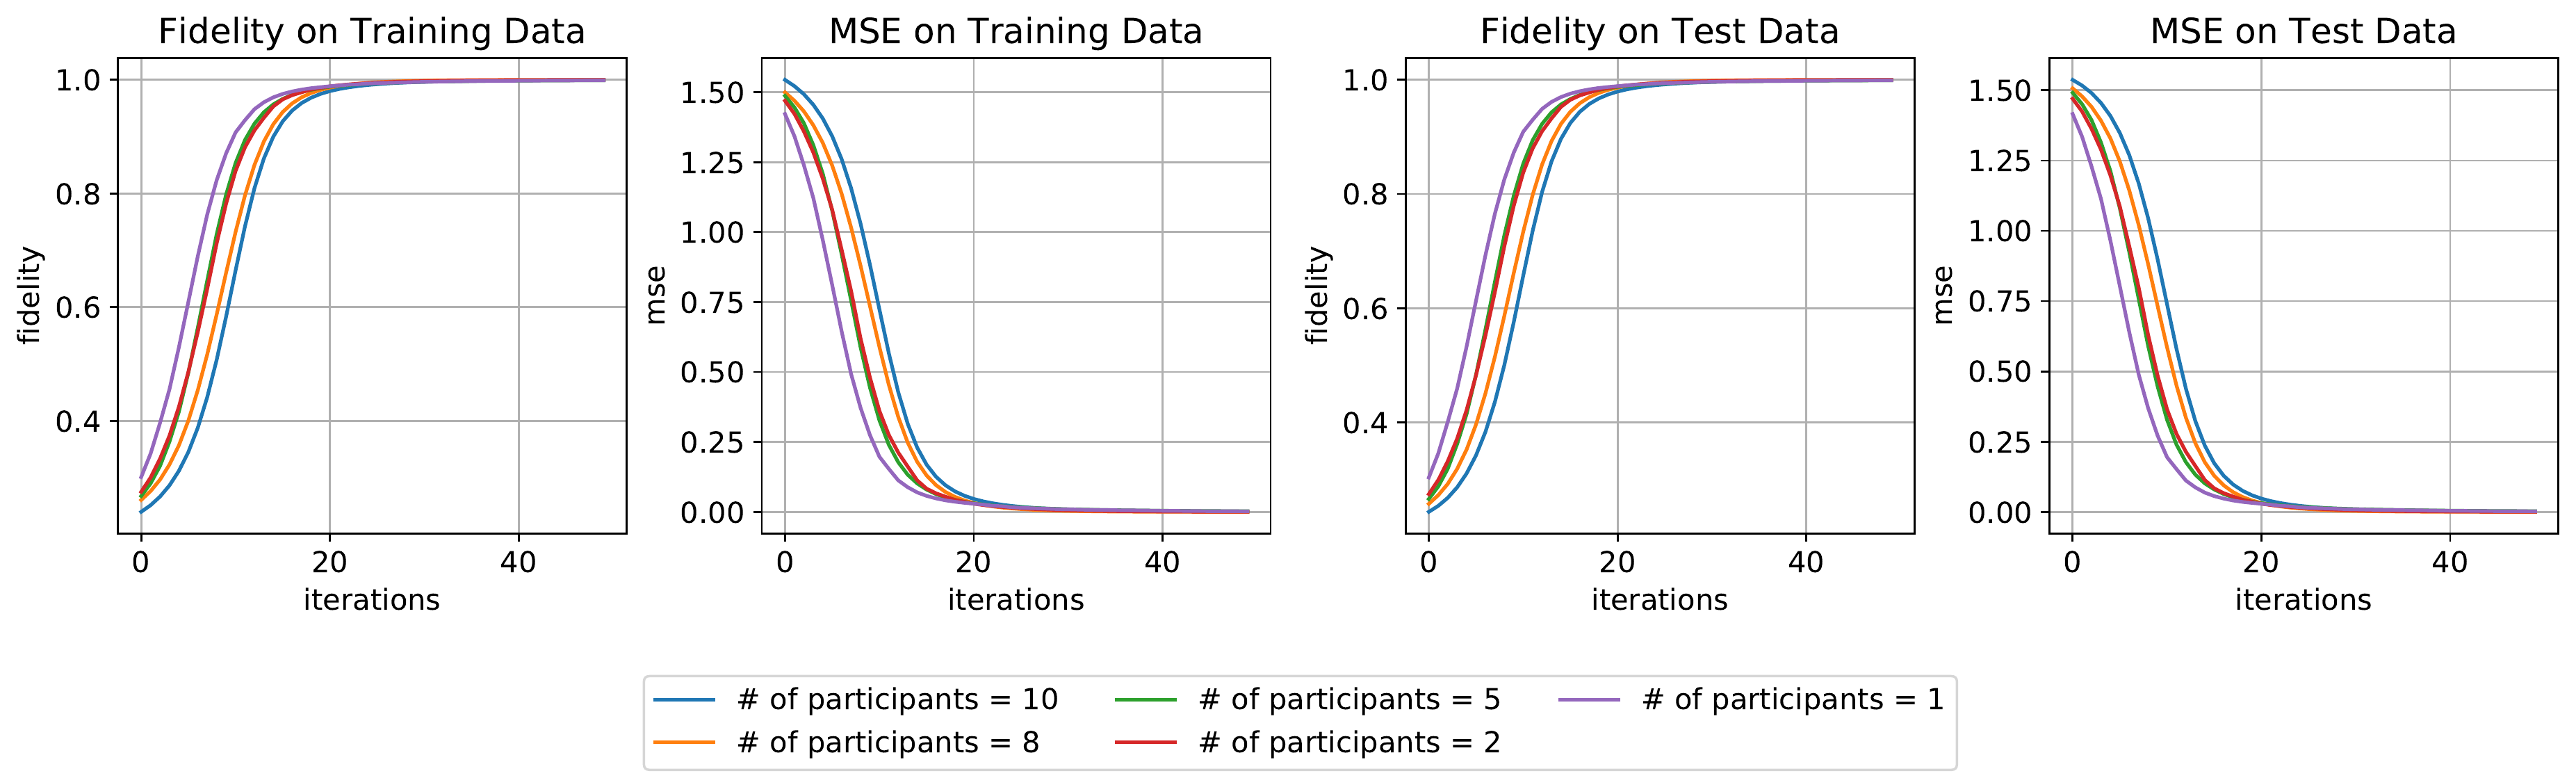}
    \caption{Experiment results of a [2, 3, 2] quantum network with different numbers of participants.}
    \label{participants_comparison}
\end{figure}
\begin{figure}[htb]
    \centering
    \includegraphics[width=\columnwidth]{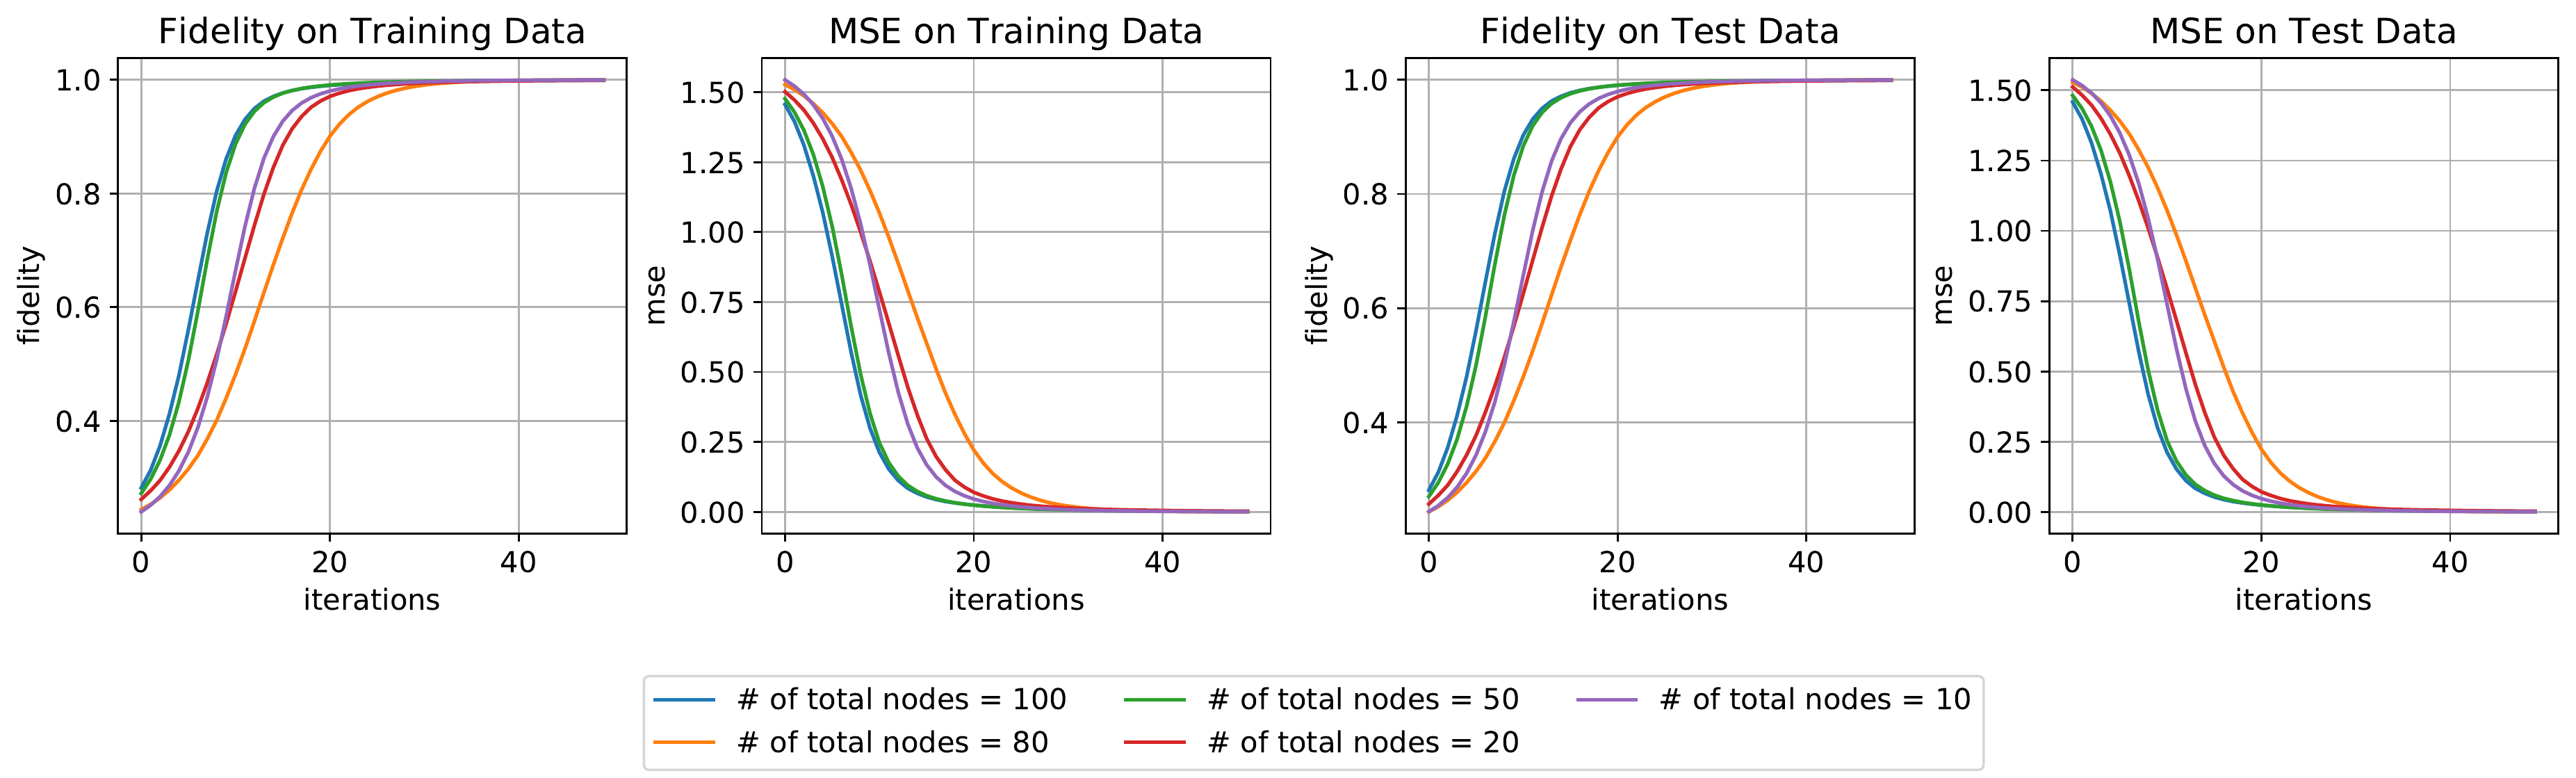}
    \caption{Experiment results of a [2, 3, 2] quantum network with different numbers of total nodes.}
    \label{totalnodes_comparison}
\end{figure}
Because the training data and test data are synthetically generated, the final performance does not vary much. However, the convergence speed does make a difference. When all of the nodes are selected to perform computations in each iteration, the convergence rate is the fastest. This is easy to understand because we got the full information of the whole dataset. Since the final performance is similar, we can choose the proportion of participants according to actual conditions in practice.
